# Supplementary material for: Digital Security -- A Question of Perspective. A Large-Scale Telephone Survey with Four At-Risk User Groups
Source: arXiv:2212.12964 source file (2023-09-12)
Supplement: Supplementary file 1 [file meta_review.tex]

\newpage % The Meta-Review should at least start on a new column

% Use \appendices and not \appendix due to IEEEtran.cls quirks
% \appendices % if not used earlier

\section{Meta-Review}

\subsection{Summary}
This papers presents a large-scale analysis of digital security experiences across four at-risk groups in Germany -- older adults, teenagers, people with low formal education, and people with a migration background. 
While all four groups experienced higher rates of cyber misuse compared to previous work on the general German population, some individual variances occurred.

\subsection{Scientific Contributions}
\begin{itemize}
\item Independent Confirmation of Important Results with Limited Prior Research
\end{itemize}

\subsection{Reasons for Acceptance}
\begin{enumerate}
\item This paper, through phone interviews with 250 people in four separate at-risk groups, provides a large-scale confirmation of previous work on these users. Crucially, it reaches far more participants than is typical for work in this field, which has primarily been limited to small-scale interview studies.
\item This paper situates its results well in comparison to prior literature. While it mostly confirms prior results on a large scale, it also offers nuance to previous findings, especially regarding who these users expect to attack them.
\end{enumerate}

\subsection{Noteworthy Concerns} % Exclude if your meta-review does not have noteworthy concerns
\begin{enumerate} % Enumerate environment is not necessary if there is only one
\item Some reviewers were concerned that this paper does not take a sample of a control group for comparison -- the paper focuses on between-group comparisons of groups that are at-risk for different reasons.
\item Due to the specific nature of the ``migrant'' category, comparison with previous work is difficult - the definition of migrant in Germany includes diverse backgrounds and timelines, compared to previous work that is more specific to, \eg, refugees and migrants under specific political pressure. 
The European Union's definition, which was used by the authors, includes groups from prior work, but also others, like citizens with just one parent born in a different country -- this is a broader criterion than most prior work.
\end{enumerate}

% \section{Response to the Meta-Review} % Optional

% Less than 500 words response to the meta-review. The response to the
% meta-review is optional. Provide a response if you disagree with the
% meta-review. Shepherds will only deny responses to meta-reviews if they are too
% long or are abusive / inappropriate.
